# Supplementary material for: CUDA Agent: Large-Scale Agentic RL for High-Performance CUDA Kernel Generation
Source: arXiv:2602.24286 source file (2026-02-27)
Supplement: Supplementary file 1 [file 3_base_model_performance.tex]

\section{Performance of the Base Model}
\label{appd:base_model_performance}

\subsection{Benchmark Descriptions}
To provide a comprehensive evaluation of our Base Model, we selected a diverse set of benchmarks covering General Knowledge, Reasoning, Math, and Coding. The details of these benchmarks are as follows:

\begin{description}
    \item[MMLU] A comprehensive test covering 57 subjects across STEM, the humanities, the social sciences, and more. It measures the model's general knowledge and problem-solving ability.
    \item[MMLU-Pro] An enhanced and more challenging version of MMLU designed to better discriminate between high-performing models, requiring more robust reasoning capabilities.
    \item[SuperGPQA] An advanced evaluation set focused on graduate-level scientific reasoning, testing the model's ability to answer complex questions in biology, physics, and chemistry.
    \item[BBH] A subset of the BIG-bench task suite, focusing on tasks where language models have historically struggled. It evaluates multi-step reasoning, logical deduction, and algorithmic thinking.
    \item[GPQA-Diamond] A highly difficult benchmark consisting of graduate-level Google-proof Q\&A questions. The "Diamond" subset represents the highest quality and hardest questions, intended to test expert-level scientific knowledge.
    \item[GSM8k] A dataset of high quality linguistically diverse grade school math word problems. It is the standard benchmark for multi-step mathematical reasoning.
    \item[MATH] A dataset of challenging mathematics problems from high school math competitions. It is significantly harder than GSM8k and requires complex problem-solving skills.
    \item[MBPP] A benchmark for evaluating code generation, consisting of crowd-sourced Python programming problems that cover programming fundamentals and standard library usage.
\end{description}

% \subsection{Performance Comparison}
% Table \ref{tab:base_model_benchmarks_v2} presents the performance of our base model compared to LLaMA-4-Maverick Base, DeepSeek-V3 Base, Qwen3-235B-A22B Base, and Kimi-K2 Base. Our base model achieves performance comparable to state-of-the-art open-source models across a diverse set of benchmarks, encompassing general knowledge, logical reasoning, STEM, mathematics, and code generation.

\begin{table}[h!]
\centering
\caption{Comparison of our Base Model with other leading base models. The best results are highlighted in \textbf{bold}. An em dash (—) indicates that the result is not reported. Kimi-K2 Base is reported to achieve 80.33 on EvalPlus (averaging HumanEval, MBPP, HumanEval+, and MBPP+).}
\label{tab:base_model_benchmarks_v2}
\resizebox{\textwidth}{!}{%
\begin{tabular}{llccccc}
\toprule
\textbf{Category} & \textbf{Benchmark} & \textbf{Base Model (Ours)} & \textbf{LLaMA-4-Maverick Base} & \textbf{DeepSeek-V3 Base} & \textbf{Qwen3-235B-A22B Base} & \textbf{Kimi-K2 Base} \\
\midrule
\multirow{4}{*}{\makecell[l]{General Knowledge \\ \& Reasoning}} 
 & MMLU & \textbf{88.83} & 85.16 & 87.19 & 87.81 & 87.79 \\
 & MMLU-Pro & \textbf{69.98} & 63.91 & 59.84 & 68.18 & 69.17 \\
 & SuperGPQA & \textbf{45.08} & 40.85 & 41.53 & 44.06 & 44.67 \\
 & BBH & \textbf{92.08} & 83.62 & 86.22 & 88.87 & 88.71 \\
\midrule
\multirow{4}{*}{\makecell[l]{STEM \& Math \\ \& Coding}} 
 & GPQA-Diamond & 43.43 & 43.94 & 41.92 & 47.47 & \textbf{48.11} \\
 & GSM8k & 93.10 & 87.72 & 87.57 & \textbf{94.39} & 92.12 \\
 & MATH & \textbf{72.86} & 63.32 & 62.62 & 71.84 & 70.22 \\
 & MBPP & \textbf{83.60} & 75.40 & 74.20 & 81.40 & – \\
\bottomrule
\end{tabular}%
}
\end{table}
